# Supplementary material for: Robust Feature Inference: A Test-time Defense Strategy using Spectral Projections
Source: arXiv:2307.11672 source file (2024-08-23)
Supplement: Supplementary file 1 [file appendix.tex]

\section{Appendix}
\subsection{Proof of Proposition~\ref{prop:ntkrfsame}}
Given our assumptions of random feature model, we know that the feature covariance matrix and NTK gram matrix are in essence dual of each other which share the eigenvalues and thus the eigenvectors can be obtained via SVD as $u_j=\frac{1
}{\sqrt{\lambda_j}}\phi(\mathcal{X})v_j$  
Then our NTK features defined using gram matrix correspond to eigenbasis features as, 
\begin{equation*}
\begin{aligned}
f^{ker}_j(x) &= \frac{1}{\lambda_j}O(x,\mathcal{X})^Tv_jv_j^T\mathcal{Y}\\
    &=\frac{1}{\lambda_j} O(x,\mathcal{X})^Tv_jv_j^T [\phi(\mathcal{X})^T\tilde{\beta}+\epsilon]\\
    &=\phi(x)u_ju_j^T\tilde{\beta} + \frac{1}{\lambda_j}O(x,\mathcal{X})^Tv_jv_j^T\epsilon\text{ }(\text{Since }u_j=\frac{1
}{\sqrt{\lambda_j}}\phi(X)v_j)\\
    &=f_j(x)+\frac{1}{\lambda_j}O(x,\mathcal{X})^Tv_jv_j^T\epsilon
\end{aligned}
\end{equation*}
This implies that, in expectation over the error $\epsilon$ we can say, 
\begin{equation*}
    \mathbb{E}_{\epsilon\sim \mathcal{N}(0,\sigma^2)}[f^{ker}_j(x)]=f_j(x)
\end{equation*}
Since $f_j(x)$ is $\rho-$useful and $\gamma-$robust it implies the NTK features also hold the same properties.  
\subsection{Proof of Theorem~\ref{theorem:gradientdescentineigenbasis}}
We use the gradient descent update rule recursively
define the evolution of $\beta$ with time steps during gradient descent as:
\begin{equation*}
    \begin{aligned}
        \beta_{t+1}&=\beta_t-\eta \nabla_\beta L\\
        &=(I-\eta\Sigma)^t\beta_0 +\sum_{k=0}^{t-1}(I-\eta\Sigma)^k\eta \alpha\\
       &=  (I-\eta\Sigma)^t\beta_0 + \Sigma^{-1}(I - (I-\eta\Sigma)^t)\alpha\\
       &= (I-\eta \Sigma)^t(\beta_0-\Sigma^{-1}\alpha)+\Sigma^{-1}\alpha
    \end{aligned}
\end{equation*}
 and $\alpha=\frac{1}{n}\phi(X)y\approx \Sigma\tilde{\beta}$.
For simplicity, it is easy to assume that $n\rightarrow\infty$ and so $\hat{\Sigma}\rightarrow\Sigma$. Recursively one can compute $\beta_t$
\begin{equation*}
\begin{aligned}
       \beta_{t+1}&= (I-\eta\Sigma)^t\beta_0 +\sum_{k=0}^{t-1}(I-\eta\Sigma)^k\eta \alpha\\
       &=  (I-\eta\Sigma)^t\beta_0 + \Sigma^{-1}(I - (I-\eta\Sigma)^t)\alpha\\
       &= (I-\eta \Sigma)^t(\beta_0-\Sigma^{-1}\alpha)+\Sigma^{-1}\alpha
\end{aligned}
\end{equation*}
Also, 
\begin{equation*}
    \begin{aligned}
        \alpha &= \frac{1}{n}\phi(X)y
               &= \frac{1}{n}\sum_{i=1}^n\phi(x_i)y_i
               &= \frac{1}{n}\sum_{i=1}^n\phi(x_i)(\phi(x_i)^T\tilde{\beta}+\epsilon_i)
               &= \hat{\Sigma}\tilde{\beta} + \sum_{i=1}^nx_i^T\epsilon_i
               &\approx \Sigma\tilde{\beta}
    \end{aligned}
\end{equation*}
And this implies,
\begin{equation*}
    \begin{aligned}
        \beta_t &= (I-\eta \Sigma)^t\beta_0+(I-(I-\eta \Sigma)^t)\tilde{\beta}\\
        &= \sum_{j=1}^p(1-\eta \lambda_j^2)^tu_ju_j^T\beta_0+
        \sum_{j=1}^p(1-(1-\eta \lambda_j^2)^t)u_ju_j^T\tilde{\beta}
    \end{aligned}
\end{equation*}
Where For any $x$,
\begin{equation*}
    \begin{aligned}
        y_t&=y_t(x)&= x^T\beta_t
        &= \sum_{j=1}^p (1-\eta\lambda_j^2)^t x^Tu_ju_j^T\beta_0+(1-(1-\eta\lambda_j^2)^t) x^Tu_ju_j^T\tilde{\beta}
    \end{aligned}
\end{equation*}
Assume, $\beta_0=0$ then $y_t(x)=\sum_{j=1}^p(1-(1-\eta\sigma_j^2)^t) x^Tu_ju_j^T\tilde{\beta}$ and $y_t(x)=\sum_{j=1}^p(1-(1-\eta\lambda_j^2)^t)f_{true}^j(x)$, where $f_{true}^j(x)=x^Tu_juj^T\tilde{\beta}$ and $f_t^j(x)=(1-(1-\eta\lambda_j^2)^t)f_{true}^j(x)$. 

Note: If $\eta\rightarrow0$ with $\tau=t\eta$ then $(1-\eta\lambda_j^2)^t\rightarrow e^{-\lambda_j^2\tau}$. Hence $f^j_t(x)=(1-e^{-\eta\lambda_j^2})f_{true}^j(x)$ but we stick with $\eta>0$ for now. Claim: Function is learned faster along the principal component. 
\begin{equation*}
    \begin{aligned}
        \%Err_j &= \frac{f_{true}^j-f_t^j}{f_{true}^j}\\
        &= (1-\eta\lambda_j^2)^t\\
        &\approx e^{-\eta\lambda_j^2}
    \end{aligned}
\end{equation*}
This implies $\%Err_1<\%Err_2<\dots$. Note: this doesn't say anything about risk / overall error.
\subsection{Proof of Proposition~\ref{prop:toparerobustanduseful}}
\subsubsection{$\rho-$usefulness $\mathbb{E}_{(x,y)}[yf^j(x)]\geq\rho$}
\begin{equation*}
\begin{aligned}
    \rho_j&=\mathbb{E}_{(x,y)}[yf^j(x)]
    =\mathbb{E}_{x}[x^T\tilde{\beta}\tilde{\beta}^Tu_ju_j^Tx(1-(1-\eta\lambda_j^2)^t)]\\
     &=\mathbb{E}_{x}[\sum_{i=1}^px^Tu_iu_i^T\tilde{\beta}\tilde{\beta}^Tu_ju_j^Tx(1-(1-\eta\lambda_j^2)^t)]\\
    &=(\tilde{\beta}_u^j)^2\lambda_j^2(1-(1-\eta\lambda_j^2)^t)
\end{aligned}    
\end{equation*}
If this is $>\rho$, then $j^{th}$ feature is useful. $\lambda_1^2\geq \lambda_2^2\geq\dots$ and thus $\rho_1\geq \rho_2\geq$. This implies that the high-variance features along the principal components of the covariance matrix are more useful. 
\subsubsection{$\gamma-$robustness $\mathbb{E}_{(x,y)}[\inf_{\delta\in \mathcal{B}(0,\Delta)}yf(x+\delta)]$}
\begin{equation*}
    \begin{aligned}
        \mathbb{E}_{(x,y)}[\inf_{\delta\in \mathcal{B}(0,\Delta)}yf_t^j(x+\delta)]&=(1-(1-\eta\lambda_j^2)^t)\mathbb{E}_{(x,\epsilon)}[\inf_{\delta\in \mathcal{B}(0,\Delta)}(\tilde{\beta}^Tx+\epsilon)\tilde{\beta}^Tu_ju_j^T(x+\delta)]\\
        &\text{Since only } \delta\text{ along }u_j\text{ matters take }\delta_u^j=\delta\in [-\Delta,+\Delta]\\
        &=(1-(1-\eta\lambda_j^2)^t)\mathbb{E}_{(x,\epsilon)}[\inf_{\delta\in (-\Delta,+\Delta)}(\tilde{\beta}^Tx+\epsilon)\tilde{\beta}_u^j(u_j^Tx+\delta)]\\
        &=(1-(1-\eta\lambda_j^2)^t)\mathbb{E}_{(x,\epsilon)}[{\beta}_u^ju_j^Tx(\tilde{\beta}^Tx+\epsilon)+\inf_{\delta}(\tilde{\beta}^Tx+\epsilon)\tilde{\beta}_u^j\delta)]\\
        &=(1-(1-\eta\lambda_j^2)^t)({\tilde{\beta}}_u^j)^2\lambda_j^2+(1-(1-\eta\lambda_j^2)^t)\mathbb{E}_{(x,\epsilon)}[\inf_{\delta}(\tilde{\beta}^Tx+\epsilon)\tilde{\beta}_u^j\delta)]\\
        &=(1-(1-\eta\lambda_j^2)^t)({\tilde{\beta}}^j)^2\sigma_j^2+(1-(1-\eta\lambda_j^2)^t).\Delta\mathbb{E}_{(x,\epsilon)}[|(\tilde{\beta}^Tx+\epsilon)\tilde{\beta}_u^j|]\\
        &=(1-(1-\eta\lambda_j^2)^t)({\tilde{\beta}}^j)^2\sigma_j^2+(1-(1-\eta\lambda_j^2)^t).\Delta\mathbb{E}_{(x,\epsilon)}[|(\tilde{\beta}^Tx+\epsilon)\tilde{\beta}_u^j|]\\
        &=(1-(1-\eta\lambda_j^2)^t)[({\tilde{\beta}}_u^j)^2\lambda_j^2-\Delta|\tilde{\beta}_u^j|\sqrt{\frac{2}{\pi}(\sigma^2+\Sigma(\tilde{\beta_u^j})^2\lambda_j^2)}
    \end{aligned}
\end{equation*}
Assuming $\tilde{\beta}_u^j=1$ and $\forall j$, $\sqrt{\frac{2}{\pi}(\sigma^2+\Sigma(\tilde{\beta_u^j})^2\lambda_j^2)}=c$ and (const).
\begin{equation*}
    \begin{aligned}
        \mathbb{E}_{(x,y)}[\inf_{\delta\in \mathcal{B}(0,\Delta)}yf_t^j(x+\delta)]&\leq (1-(1-\eta\lambda_j^2)^t)[\lambda_j^2-\Delta.c]
    \end{aligned}
\end{equation*}
Every $\rho-$ useful feature is $\rho-\Delta c+\Delta c(1-\eta\lambda_j^2)^t\geq \rho-\Delta c$ which is $\gamma$-robust. Similar conclusion as before that, top-few features are $\rho-$useful and $\gamma-$robust.
\subsection{Proof of Theorem~\ref{theorem:ntkfeaturefirstlearned}}
\begin{equation}
\begin{aligned}
    f(x)_{t} &= \sum_{i=0}^{n}\lambda_{i}^{-1}\mathcal{O}(x,\mathcal{X})^{T} v_iv_i^{T}(I-e^{-\gamma t\sum_{i=0}^{n}\lambda_i v_iv_i^{T}})\mathcal{Y}\\
    &= \sum_{i=0}^{n}\lambda_{i}^{-1}\mathcal{O}(x,\mathcal{X})^{T} v_iv_i^{T}(I-e^{-\gamma t}e^{\sum_{i=0}^{n}\lambda_i v_iv_i^{T}})\mathcal{Y}\\
    &= \sum_{i=0}^{n}f_{(i)}(x)-e^{-\gamma t}\sum_{i=0}^{n}\lambda_{i}^{-1}\mathcal{O}(x,\mathcal{X})^{T} v_iv_i^{T}e^{\sum_{i=0}^{n}\lambda_i v_iv_i^{T}}\mathcal{Y}\\
    &= \sum_{i=0}^{n}f_{(i)}(x)-e^{-\gamma t}\sum_{i=0}^{n}\lambda_{i}^{-1}\mathcal{O}(x,\mathcal{X})^{T} v_iv_i^{T}e^{\sum_{i=0}^{n}\lambda_i v_iv_i^{T}}\mathcal{Y}\\
    &= \sum_{i=0}^{n}f_{(i)}(x)-e^{-\gamma t}\sum_{i=0}^{n}\lambda_{i}^{-1}\mathcal{O}(x,\mathcal{X})^{T} v_iv_i^{T}\sum_{k=0}^{\infty}\sum_{j=0}^{n}\frac{\lambda_j^k}{k!}v_jv_j^{T}\mathcal{Y}\\
    &= \sum_{i=0}^{n}f_{(i)}(x)-e^{-\gamma t}\sum_{i=0}^{n}\sum_{j=0}^{n}\sum_{k=0}^{\infty}\frac{\lambda_{i}^{-1}\lambda_j^k}{k!}\mathcal{O}(x,\mathcal{X})^{T} v_iv_i^{T} v_jv_j^{T}\mathcal{Y}\\
    &= \sum_{i=0}^{n}f_{(i)}(x)-e^{-\gamma t}\sum_{i=0}^{n}\sum_{j=0}^{n}\sum_{k=0}^{\infty}\frac{\lambda_{i}^{-1}\lambda_j^k}{k!}\mathcal{O}(x,\mathcal{X})^{T} v_i\delta_{ij}v_j^{T}\mathcal{Y}\\
    &= \sum_{i=0}^{n}f_{(i)}(x)-e^{-\gamma t}\sum_{i=0}^{n}\sum_{k=0}^{\infty}\frac{\lambda_{i}^{-1}\lambda_i^k}{k!}\mathcal{O}(x,\mathcal{X})^{T} v_iv_i^{T}\mathcal{Y}\\
    &= \sum_{i=0}^{n}f_{(i)}(x)-e^{-\gamma t}\sum_{i=0}^{n}\sum_{k=0}^{\infty}\frac{\lambda_i^k}{k!}f_{(i)}(x)\\
    &= \sum_{i=0}^{n}f_{(i)}(x)-e^{-\gamma t}\sum_{i=0}^{n}e^{\lambda_i}f_{(i)}(x)\\
    &= \sum_{i=0}^{n}f_{(i)}(x)(1-e^{-\gamma t\lambda_i})\\
\end{aligned}
\end{equation}

\subsection{Risk order for features}
Recall $x\sim N(0,\Sigma^2)$, $\epsilon\in N(0,\sigma^2)$ and $y=\tilde{\beta}^TX+\epsilon$. 
\begin{equation*}
    \begin{aligned}
        \mathbb{E}_{(x,y)}[(y-y_t)^2]&=\mathbb{E}_{(x,\epsilon)}[((\tilde{\beta}^TX-y_t)+\epsilon)^2]\\
        &= \sigma^2+ \mathbb{E}_{x}[(\sum_{j=1}^p\tilde{\beta}^Tu_ju_j^Tx-y_t^j)^2]\\
        &= \sigma^2+ \mathbb{E}_{x}[(\sum_{j=1}^p\tilde{\beta}^Tu_ju_j^Tx(1-\lambda_j^2)^t)^2]\\
        &= \sigma^2+ \sum_{j=1}^p(\tilde{\beta}_u^j)^2\lambda_j^2(1-\lambda_j^2)^{2t}\\
    \end{aligned}
\end{equation*}
We define $\%risk_j=(\tilde{\beta}_u^j)^2\lambda_j^2(1-\eta\lambda_j^2)^{2t}$, where $\tilde{\beta}_u^j$ are the coefficients in the eigenbasis. Assuming $\beta_u^j=1$ $\forall j$. For $t<\frac{1}{2}(\frac{1}{\eta \lambda_1^2}-1)$ we obtain $\%risk_1>\%risk_2>\dots$. Similarly for For $t>\frac{1}{2}(\frac{1}{\eta \lambda_p^2}-1)$  we obtain $\%risk_1<\%risk_2<\dots$.
\\
Considering the rate of change of $\%risk$ as
\begin{equation*}
    \begin{aligned}
        \frac{d}{d\lambda}[\lambda(1-\eta\lambda)^{2t}]&= (1-\eta\lambda)^{2t} - 2t\eta\lambda (1-\eta\lambda)^{2t-1}\\
        &= (1-\eta\lambda)^{2t-1}(1-(2t+1)\eta\lambda)
    \end{aligned}
\end{equation*}
$\mathop{\gtrless}0$ for $t\mathop{\lessgtr}\frac{1}{2}(\frac{1}{\eta\lambda}-1)$. 
Considering $\eta\rightarrow0$ and $\tau=t\eta$. 
\begin{equation*}
    \begin{aligned}
        \frac{d}{d\lambda}[\lambda e^{-2\lambda\tau}]&= 
        &= e^{-2\lambda\tau}(1-2\lambda\tau)
    \end{aligned}
\end{equation*}
Then $\mathop{\gtrless}0$ for $\tau \mathop{\lessgtr}\frac{1}{2\lambda}$.
